# Supplementary material for: Reducing Access Disparities in Networks using Edge Augmentation
Source: arXiv:2209.07616 source file (2022-09-15)
Supplement: Supplementary file 1 [file appendix.tex]

\section{Appendix}

\label{sec:appendix}

\begin{figure*}
  \centering
\begin{subfigure}[t]{.4\textwidth}
  \includegraphics[width=\columnwidth]{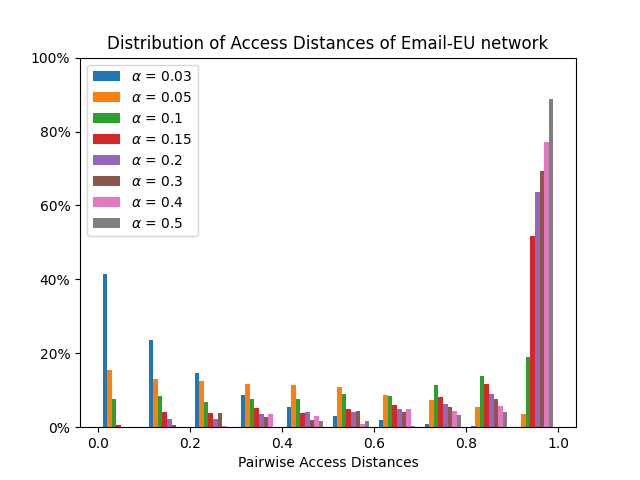}
  \caption{Email-EU}
\end{subfigure}
\begin{subfigure}[t]{.4\textwidth}
  \centering
  \includegraphics[width=\columnwidth]{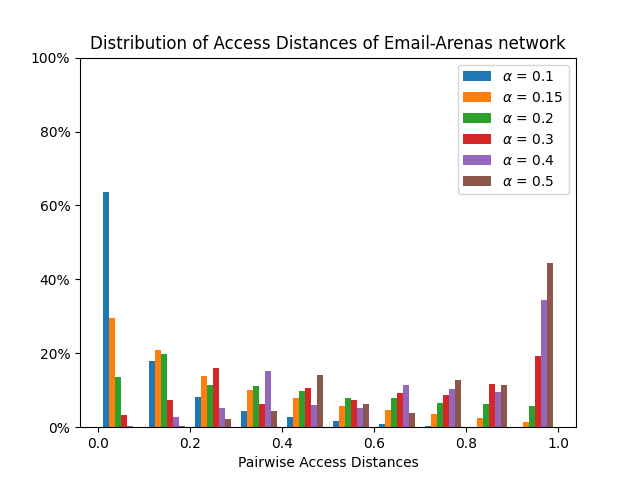}
  \caption{Email-arenas}
\end{subfigure}

\begin{subfigure}[t]{.4\textwidth}
  \includegraphics[width=\columnwidth]{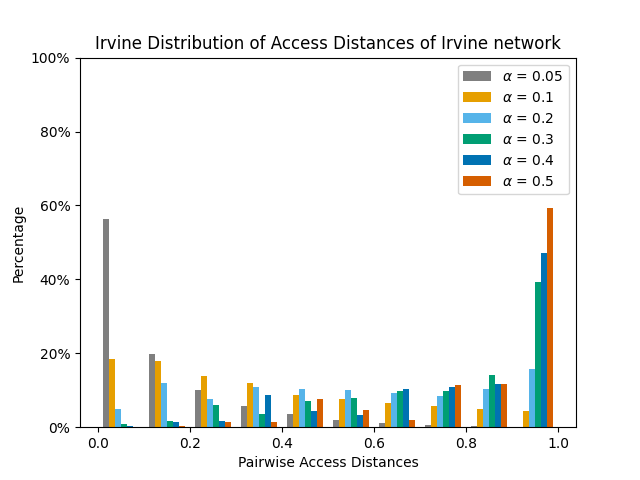}
  \caption{Irvine}
\end{subfigure}
\begin{subfigure}[t]{.4\textwidth}
  \centering
  \includegraphics[width=\columnwidth]{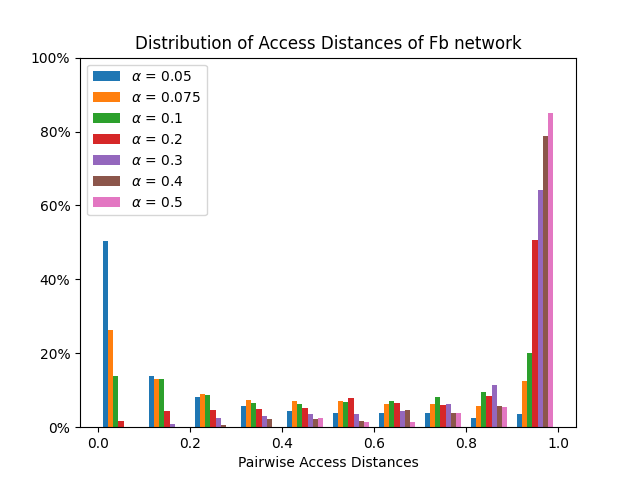}
  \caption{Facebook}
\end{subfigure}
\caption{Distribution of access probabilities for different values of $\alpha$.}
\label{fig:prob-dists}
\end{figure*}

%%%%%%%%%%%%%%%%%%%%%%%%%%%%
%%%%%%%%%%%%%%%%%%%%%%%%%%%%
%%%%%%%%%%%%%%%%%%%%%%%%%%%%

\begin{figure*}
	\centering
	\begin{subfigure}[t]{\textwidth}
		\includegraphics[width=.24\columnwidth]{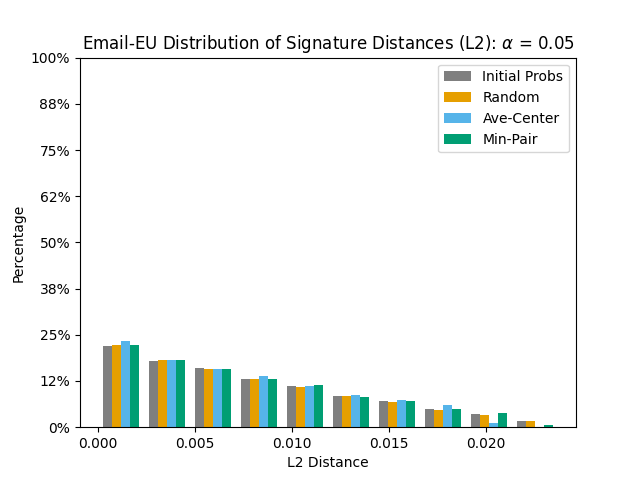}
		\includegraphics[width=.24\columnwidth]{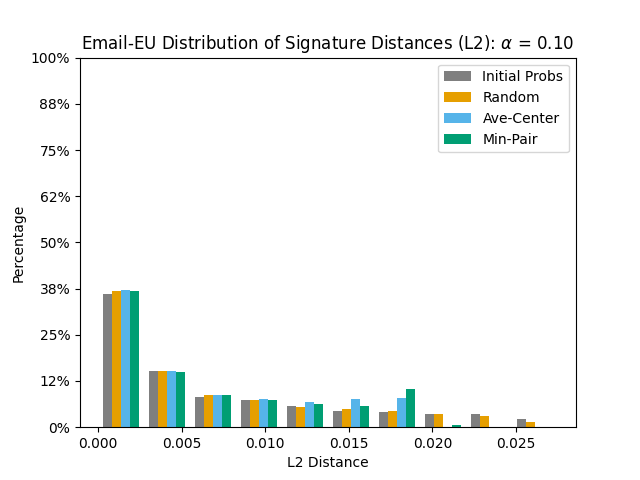}
		\includegraphics[width=.24\columnwidth]{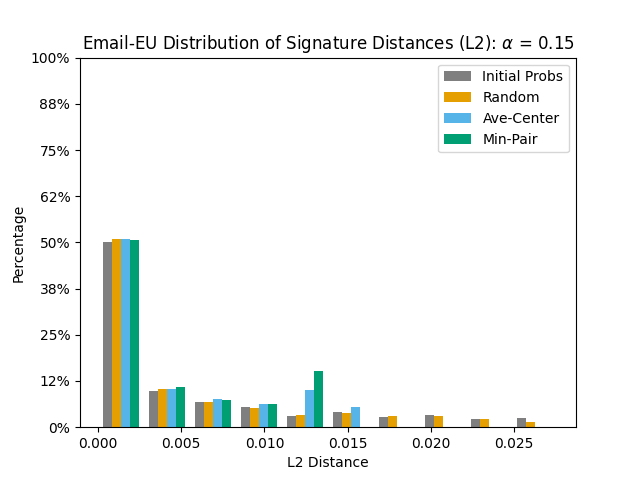}
		\includegraphics[width=.24\columnwidth]{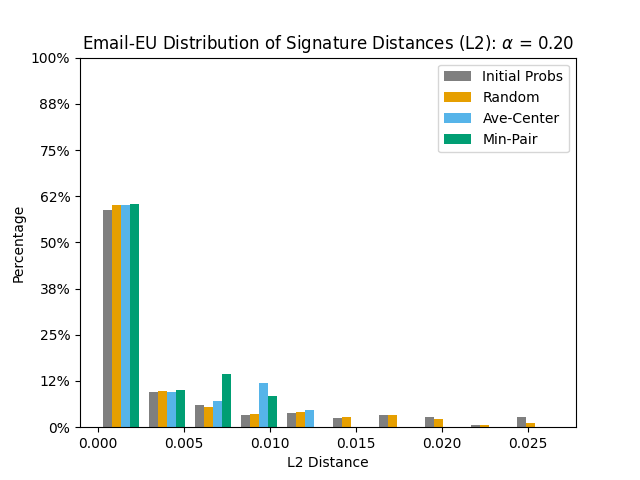}
		\caption{Email-EU}
	\end{subfigure}

	\begin{subfigure}[t]{\textwidth}
 		\includegraphics[width=.24\columnwidth]{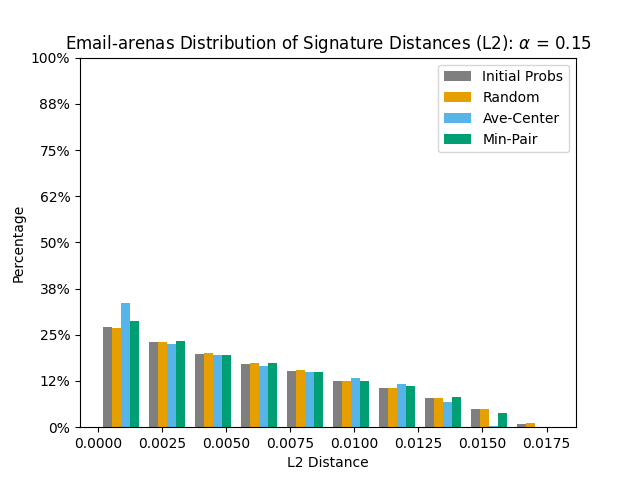}
 		\includegraphics[width=.24\columnwidth]{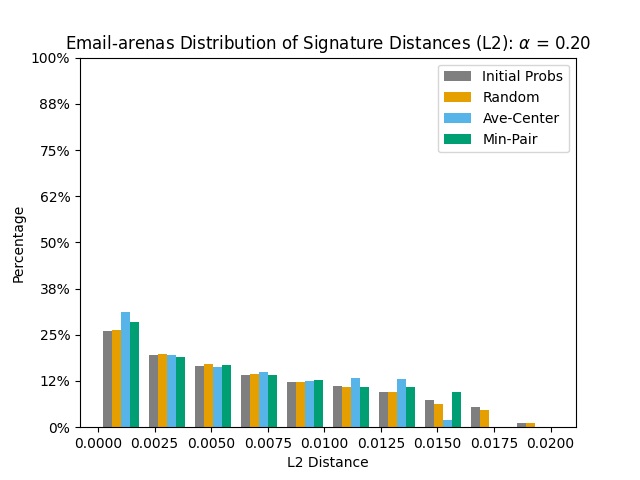}
		\includegraphics[width=.24\columnwidth]{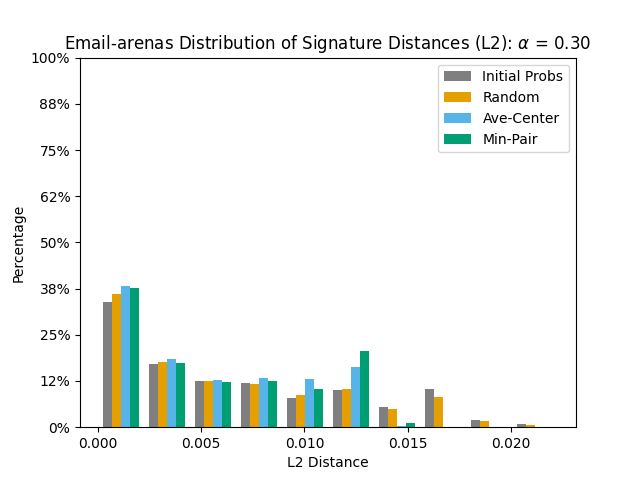}
		\includegraphics[width=.24\columnwidth]{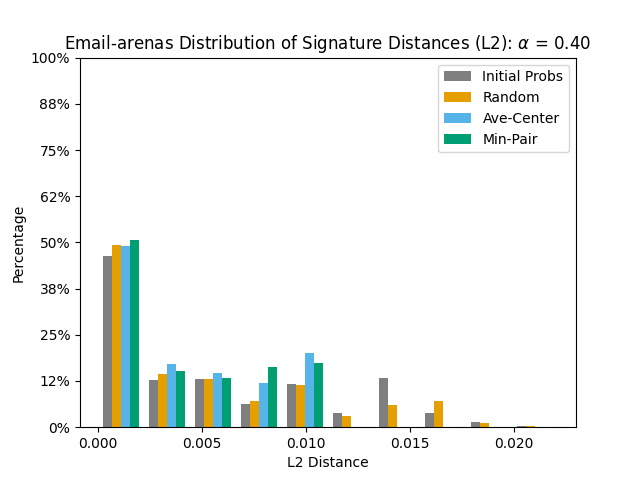}
		\caption{Email-arenas}
	\end{subfigure}

	\begin{subfigure}[t]{\textwidth}
  		\includegraphics[width=.24\columnwidth]{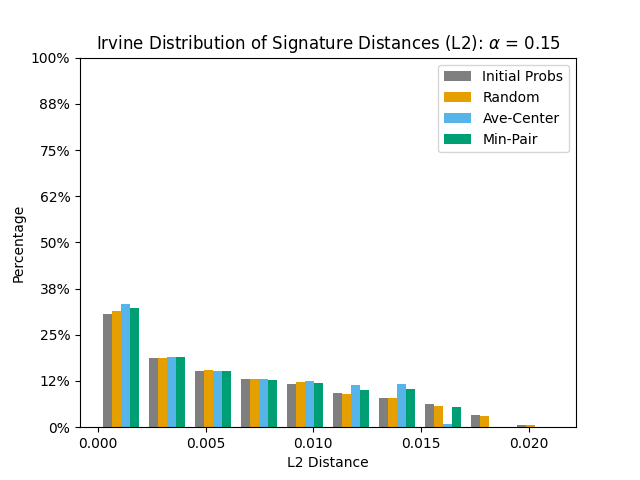}
		\includegraphics[width=.24\columnwidth]{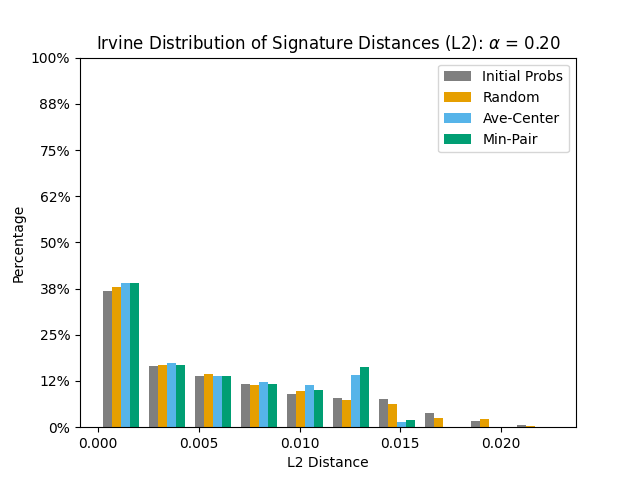}
		\includegraphics[width=.24\columnwidth]{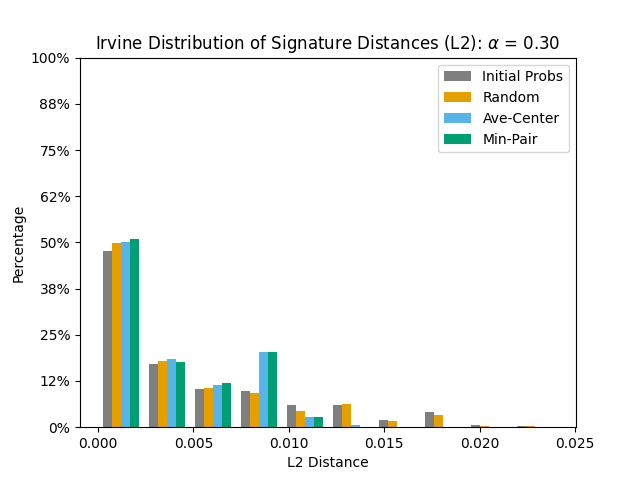}
		\includegraphics[width=.24\columnwidth]{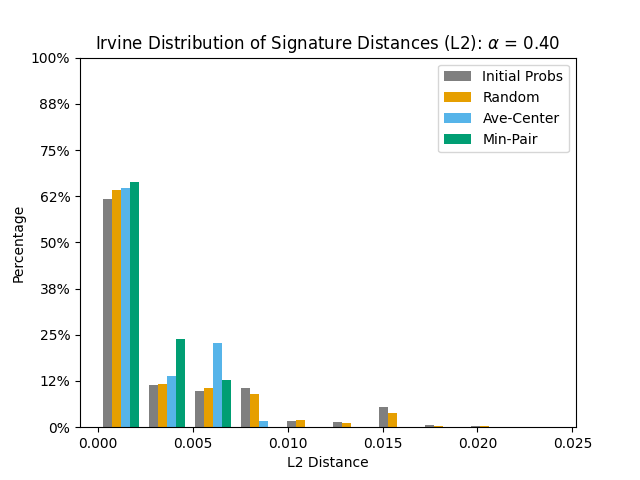}
		 \caption{Irvine}
	\end{subfigure}

	\caption{Shift in the distribution of signature euclidean distances.}
	\label{fig:sig-dist-euclid}
\end{figure*}

\begin{figure*}
	\centering
	\begin{subfigure}[t]{\textwidth}
		\includegraphics[width=.18\columnwidth]{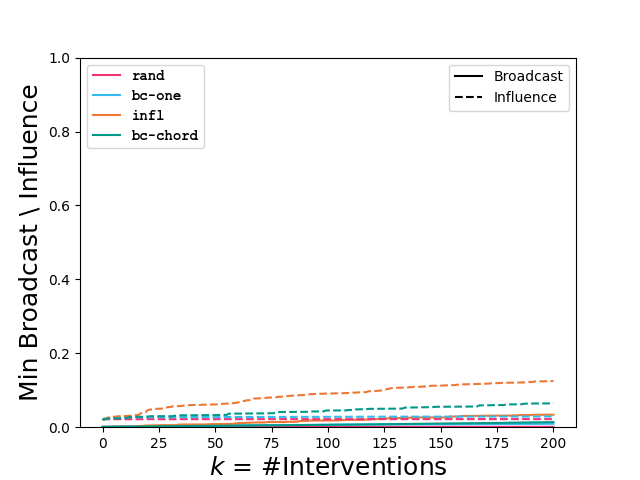}
		\includegraphics[width=.18\columnwidth]{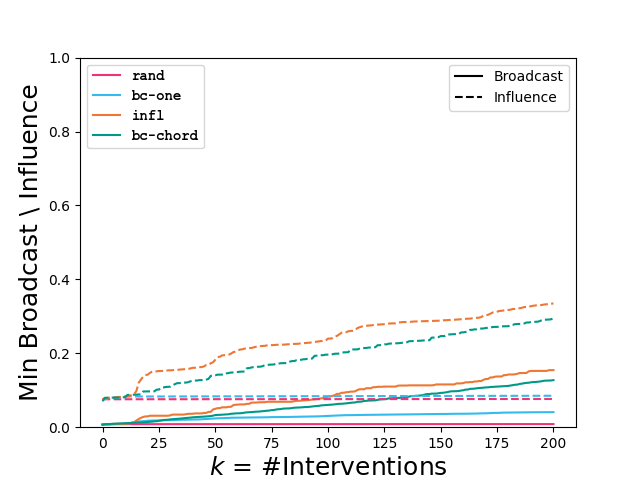}
		\includegraphics[width=.18\columnwidth]{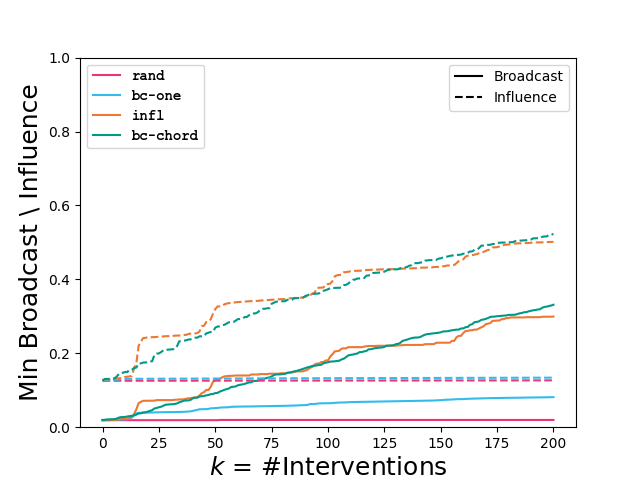}
		\includegraphics[width=.18\columnwidth]{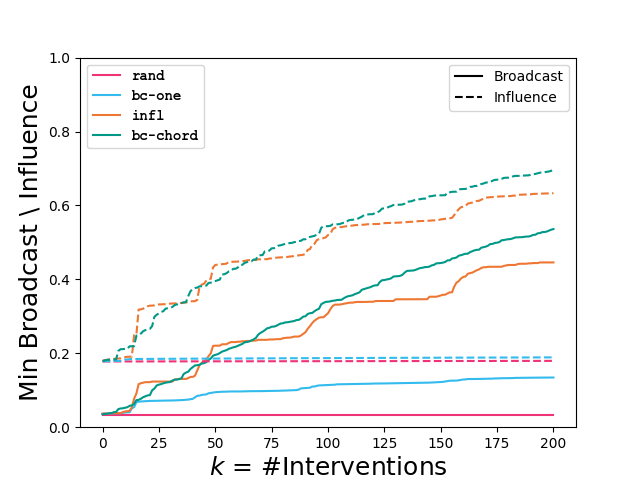}
		\includegraphics[width=.18\columnwidth]{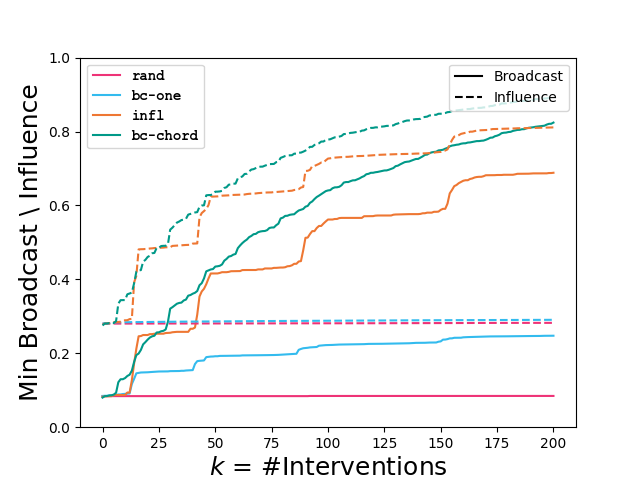}
		\caption{Email-EU}
	\end{subfigure}

	\begin{subfigure}[t]{\textwidth}
 		\includegraphics[width=.18\columnwidth]{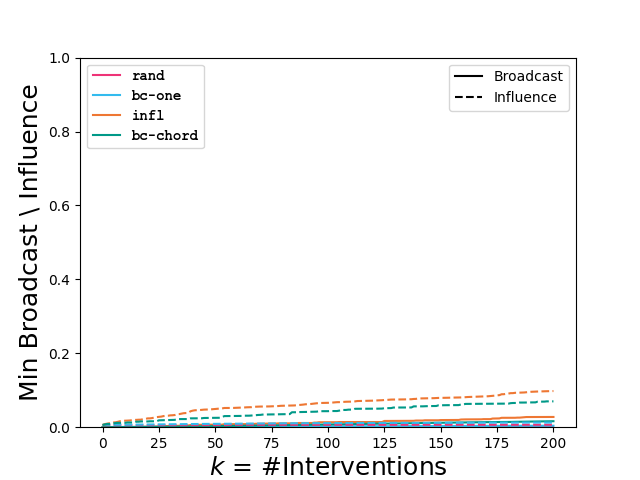}
		\includegraphics[width=.18\columnwidth]{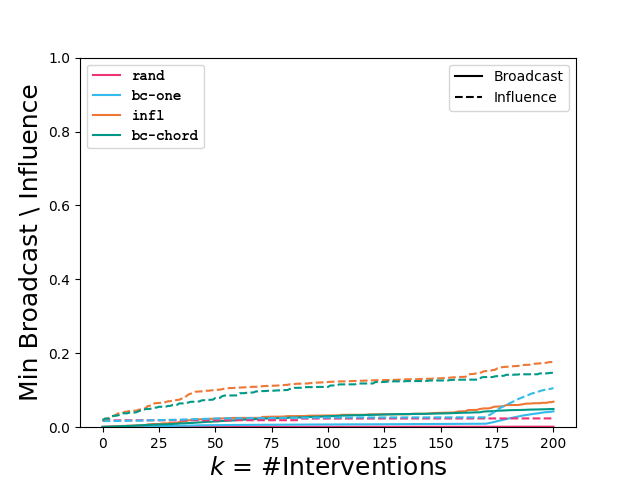}
		\includegraphics[width=.18\columnwidth]{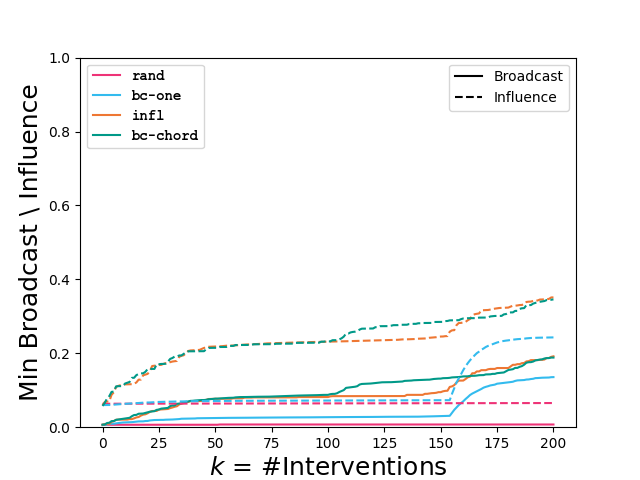}
 		\includegraphics[width=.18\columnwidth]{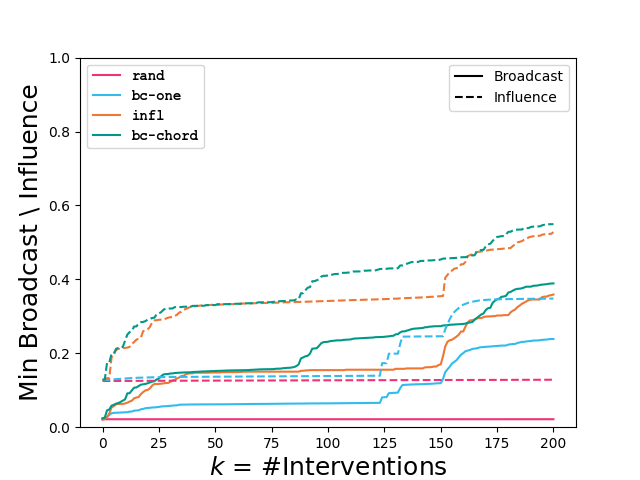}
		\includegraphics[width=.18\columnwidth]{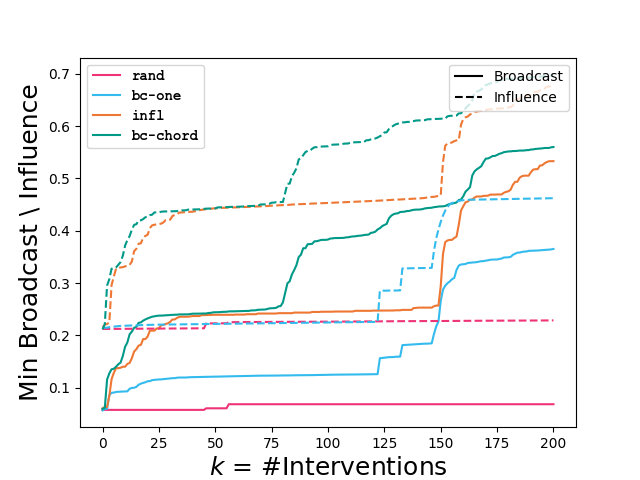}
		\caption{Email-arenas}
	\end{subfigure}

	\begin{subfigure}[t]{\textwidth}
  		\includegraphics[width=.18\columnwidth]{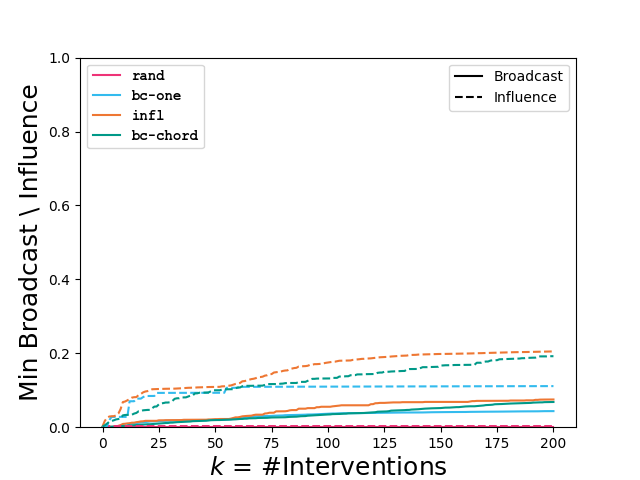}
		\includegraphics[width=.18\columnwidth]{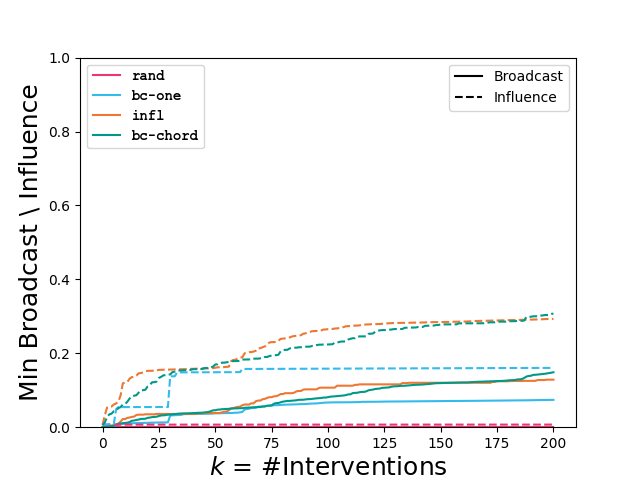}
		\includegraphics[width=.18\columnwidth]{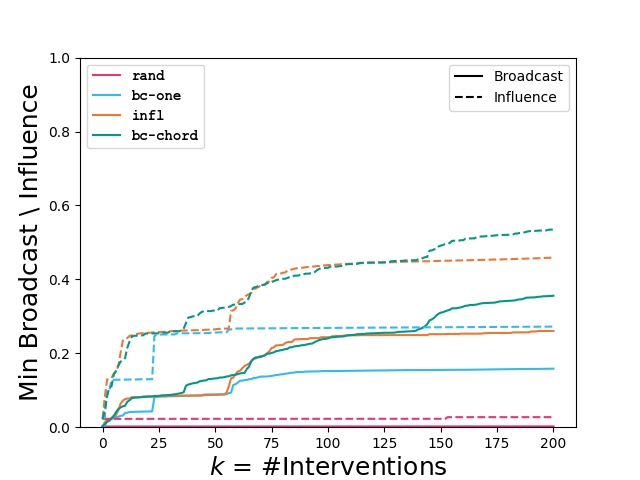}
		\includegraphics[width=.18\columnwidth]{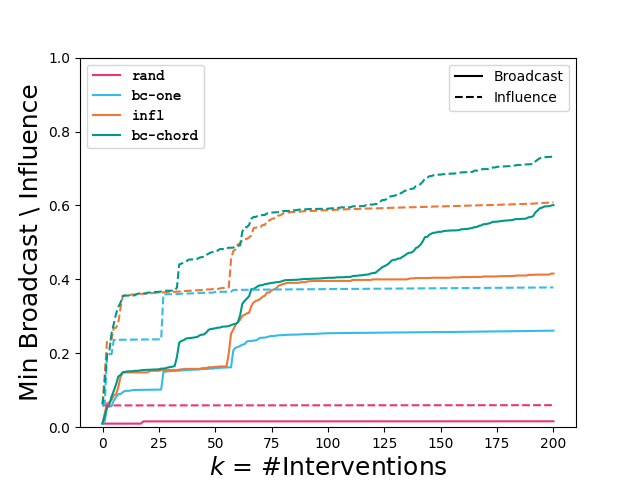}
		\includegraphics[width=.18\columnwidth]{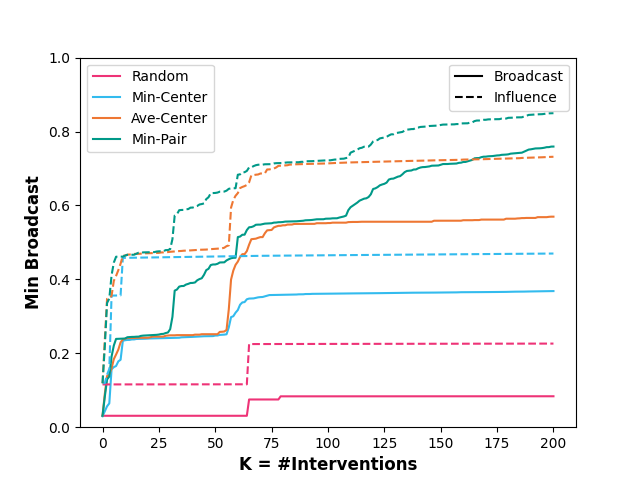}
		 \caption{Irvine}
	\end{subfigure}
	
	\begin{subfigure}[t]{\textwidth}
  		\includegraphics[width=.18\columnwidth]{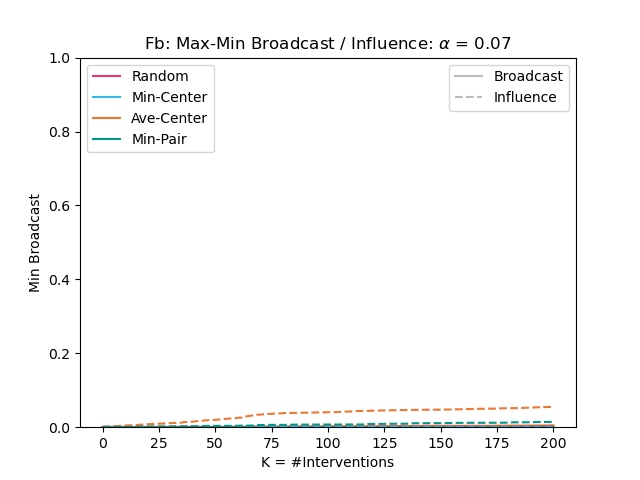}
		\includegraphics[width=.18\columnwidth]{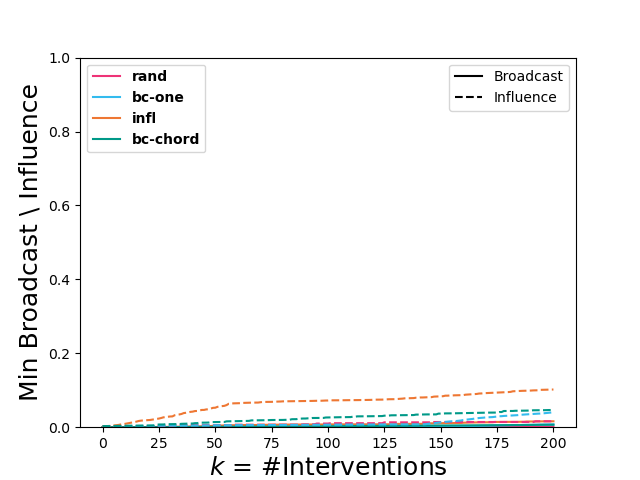}
		\includegraphics[width=.18\columnwidth]{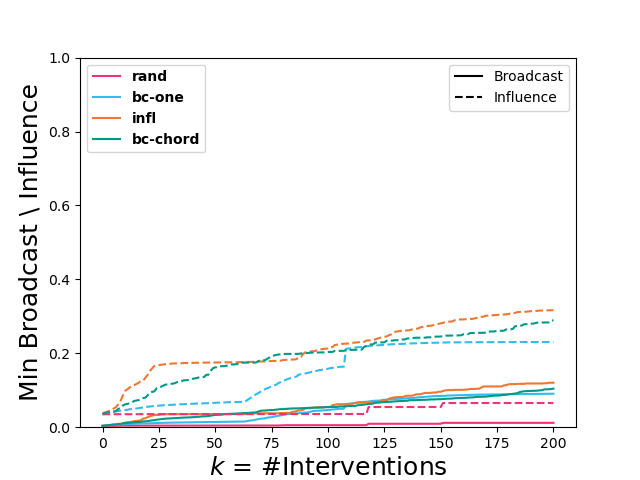}
		\includegraphics[width=.18\columnwidth]{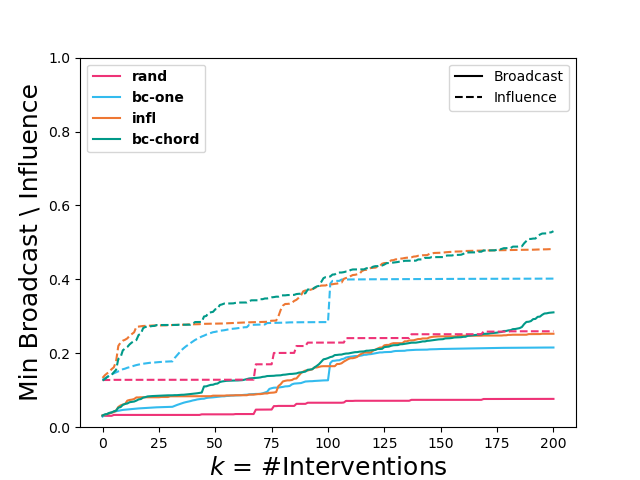}
		\includegraphics[width=.18\columnwidth]{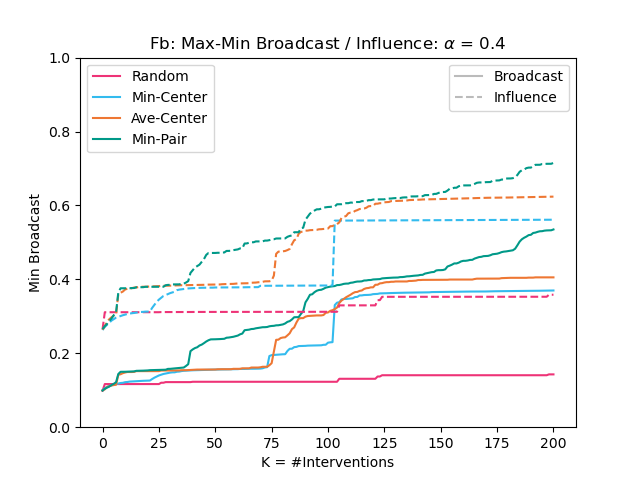}
		 \caption{Facebook}
	\end{subfigure}
	
	\begin{subfigure}[t]{\textwidth}
  		\includegraphics[width=.24\columnwidth]{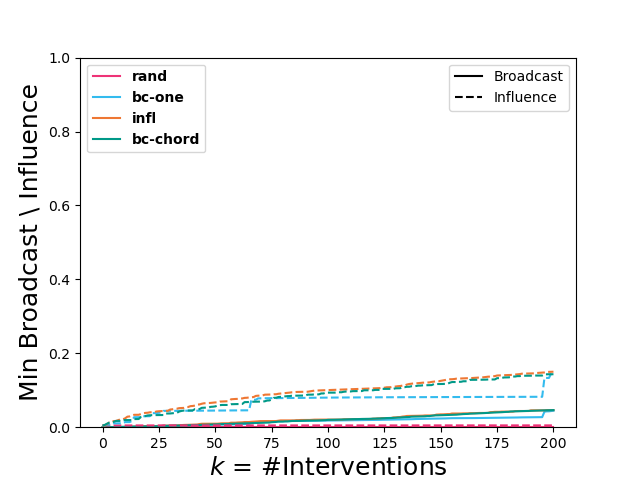}
		\includegraphics[width=.24\columnwidth]{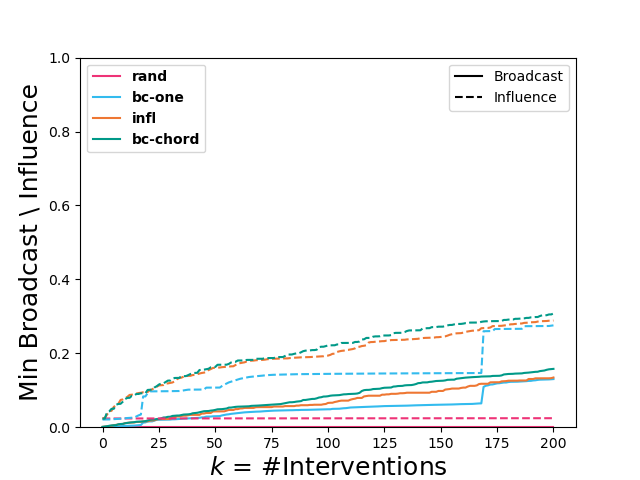}
		\includegraphics[width=.24\columnwidth]{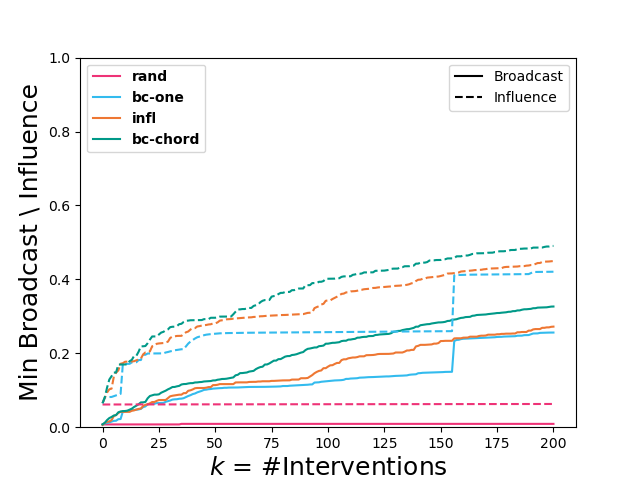}
		\includegraphics[width=.24\columnwidth]{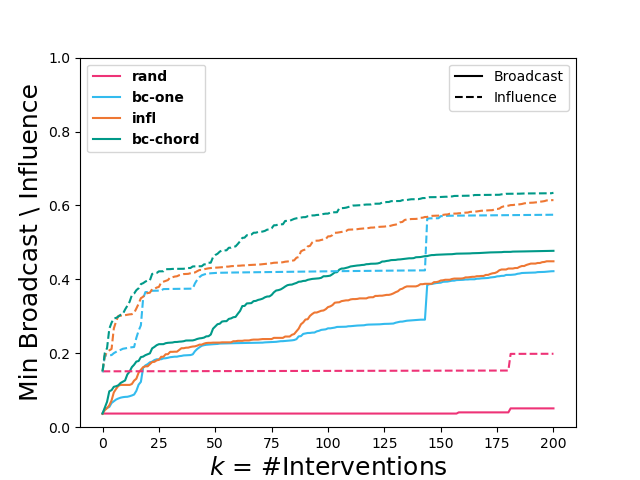}
		 \caption{Arxiv-3}
	\end{subfigure}
	
	\begin{subfigure}[t]{\textwidth}
  		\includegraphics[width=.24\columnwidth]{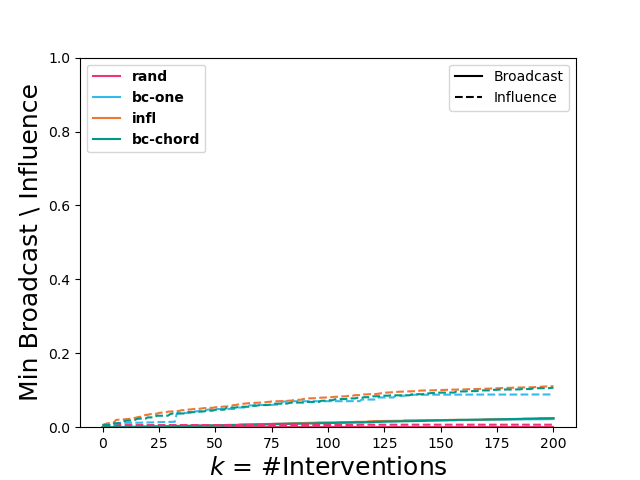}
		\includegraphics[width=.24\columnwidth]{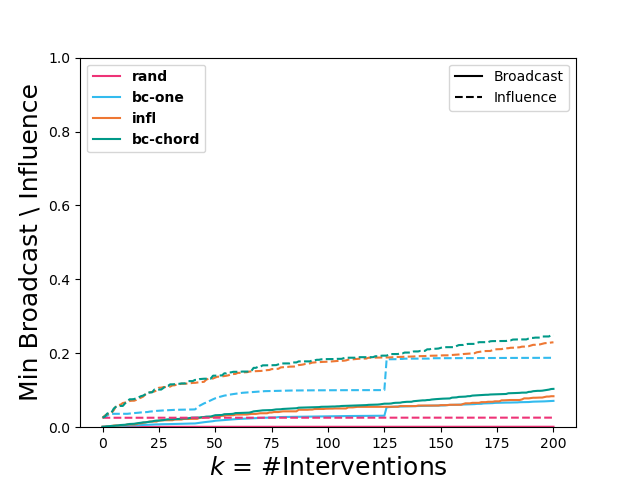}
		\includegraphics[width=.24\columnwidth]{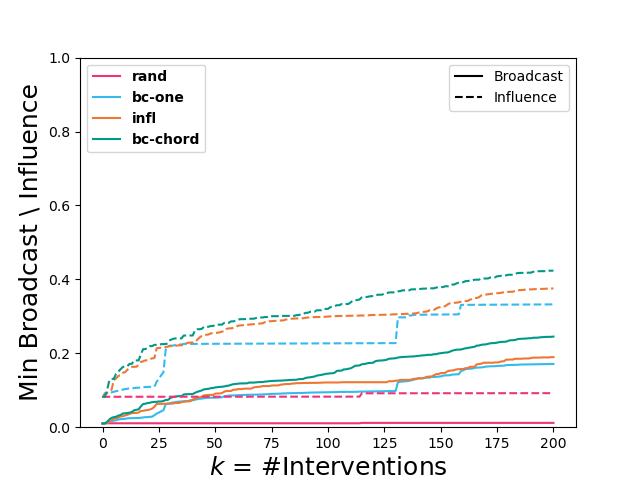}
		\includegraphics[width=.24\columnwidth]{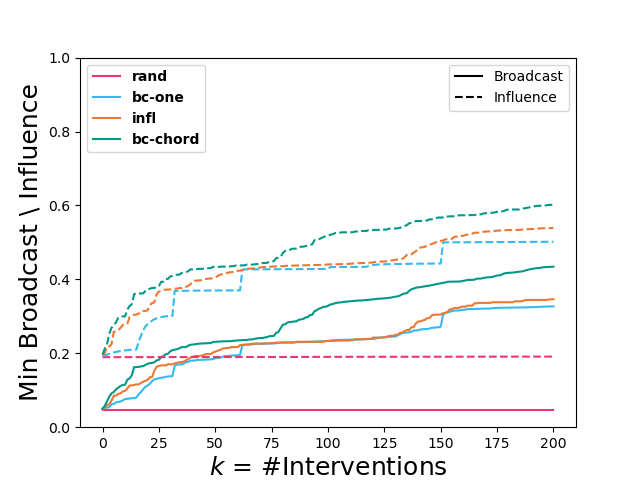}
		 \caption{Arxiv-5}
	\end{subfigure}

	\caption{Performance comparison of algorithms on maximizing the minimum \minadv{} \ \aveadv{}.}
	\label{fig:min-compare}
\end{figure*}

\begin{figure*}
	\centering
	\begin{subfigure}[t]{\textwidth}
		\includegraphics[width=.18\columnwidth]{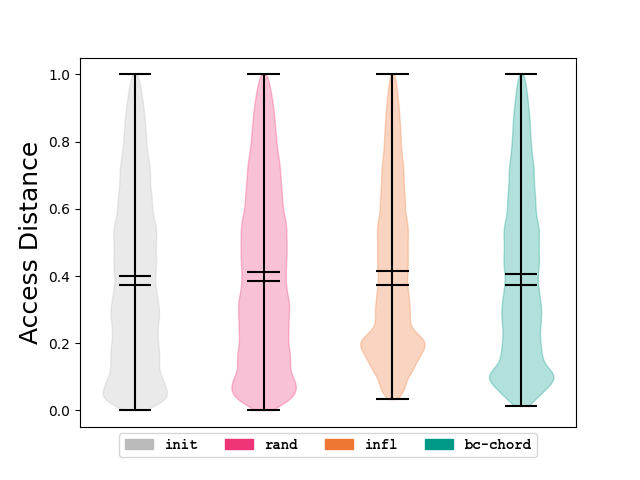}
		\includegraphics[width=.18\columnwidth]{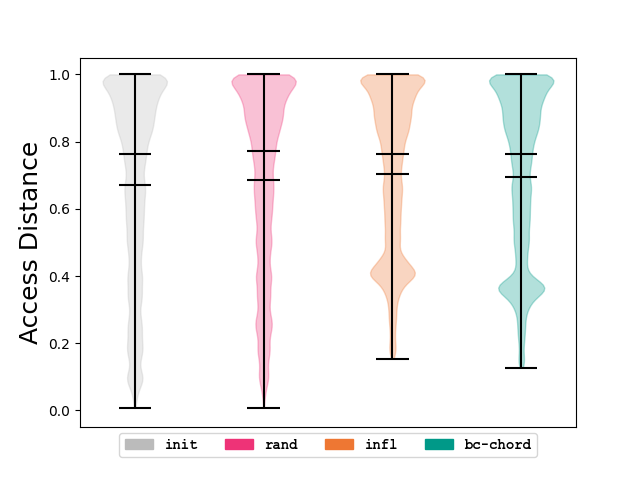}
		\includegraphics[width=.18\columnwidth]{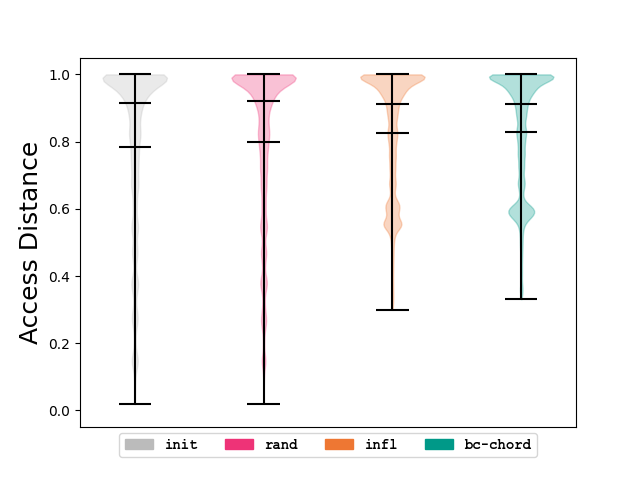}
		\includegraphics[width=.18\columnwidth]{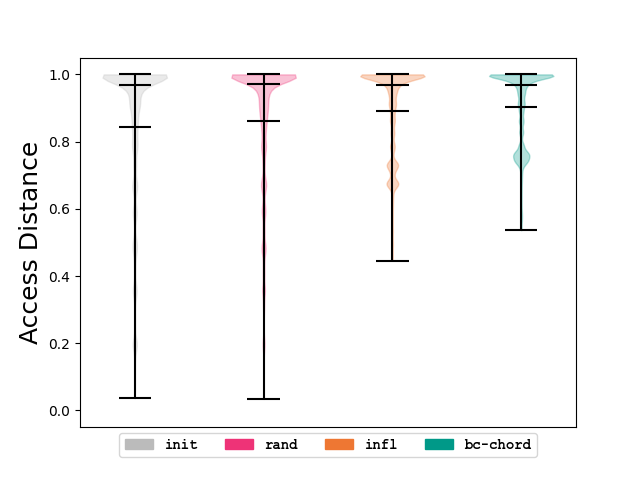}
		\includegraphics[width=.18\columnwidth]{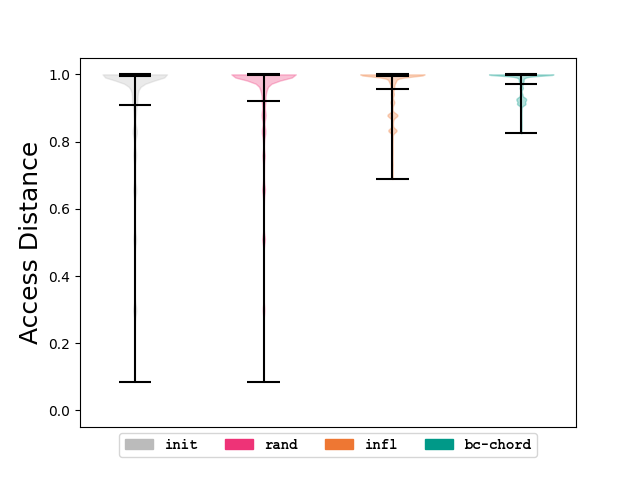}
		\caption{Email-EU}
	\end{subfigure}

	\begin{subfigure}[t]{\textwidth}
 		\includegraphics[width=.18\columnwidth]{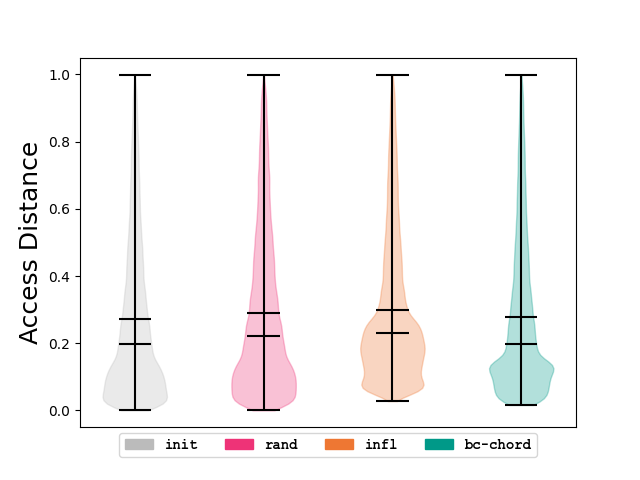}
 		\includegraphics[width=.18\columnwidth]{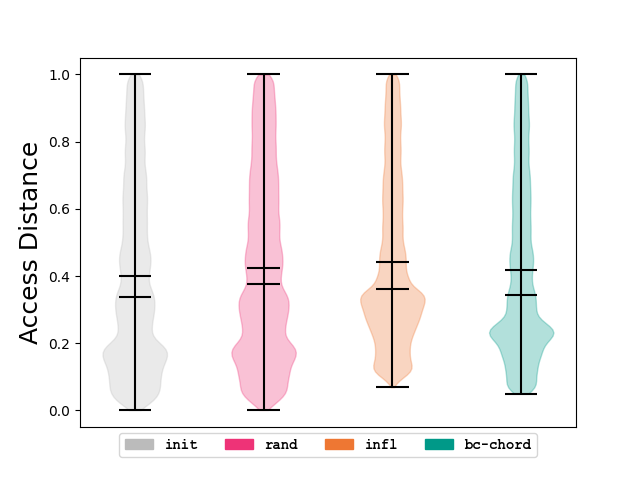}
		\includegraphics[width=.18\columnwidth]{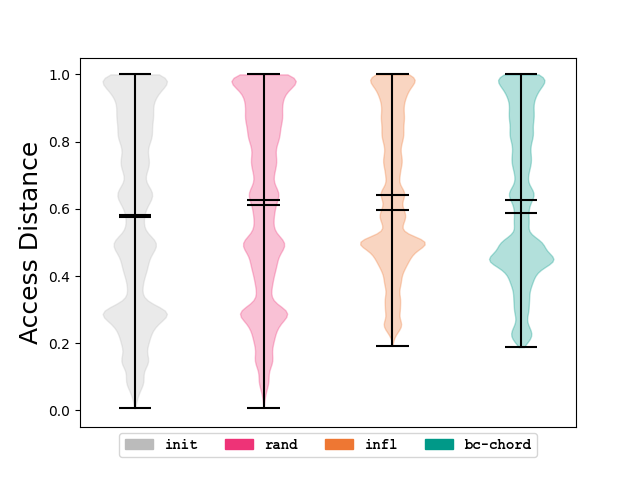}
		\includegraphics[width=.18\columnwidth]{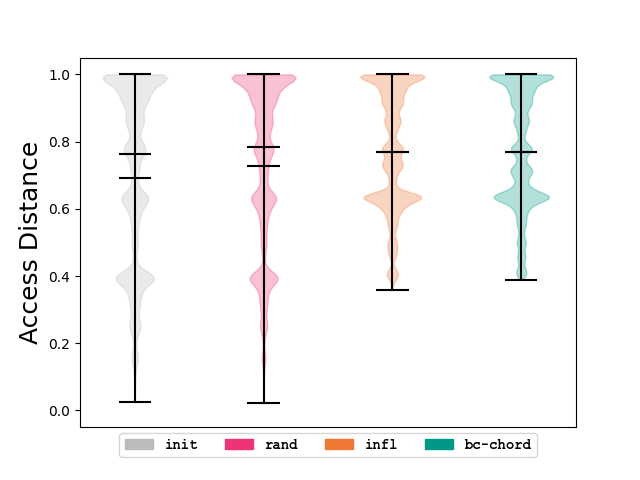}
		\includegraphics[width=.18\columnwidth]{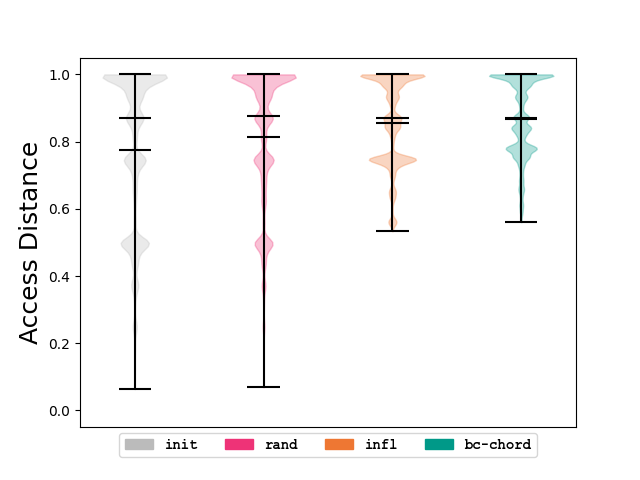}
		\caption{Email-arenas}
	\end{subfigure}

	\begin{subfigure}[t]{\textwidth}
  		\includegraphics[width=.18\columnwidth]{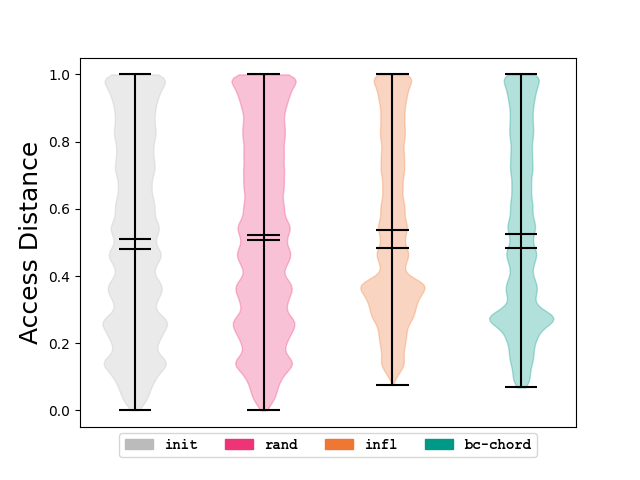}
		\includegraphics[width=.18\columnwidth]{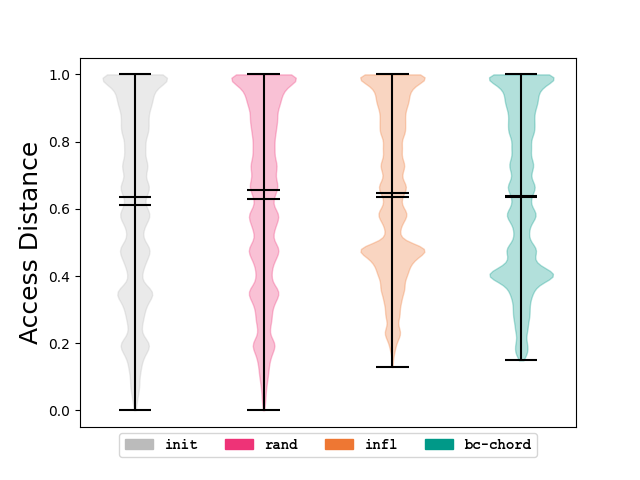}
		\includegraphics[width=.18\columnwidth]{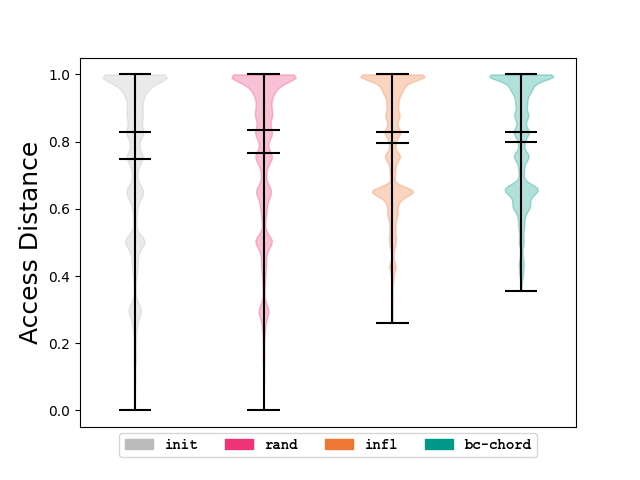}
		\includegraphics[width=.18\columnwidth]{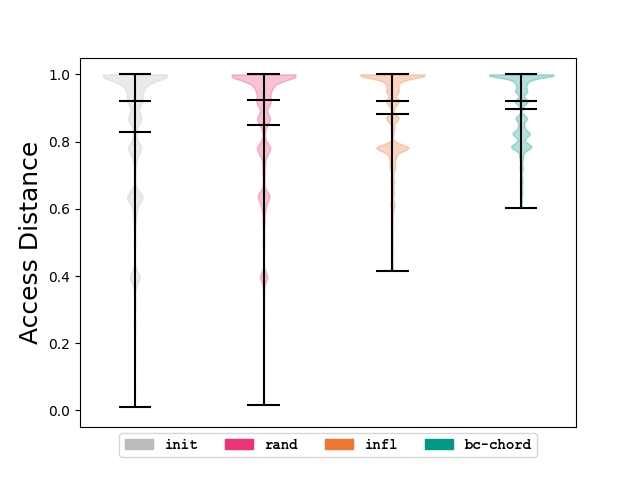}
		\includegraphics[width=.18\columnwidth]{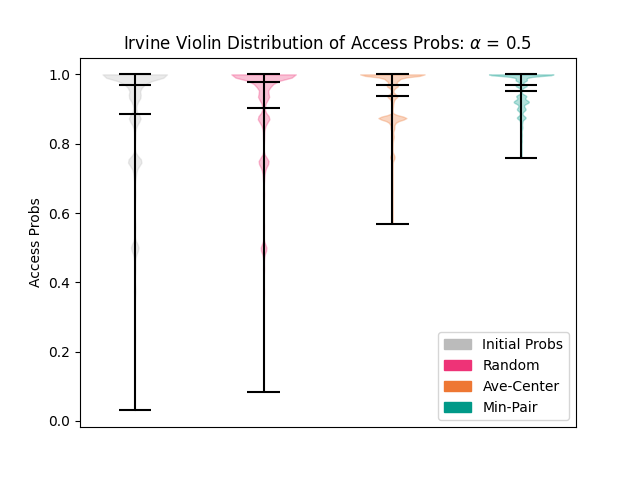}
		 \caption{Irvine}
	\end{subfigure}
	
	\begin{subfigure}[t]{\textwidth}
  		\includegraphics[width=.18\columnwidth]{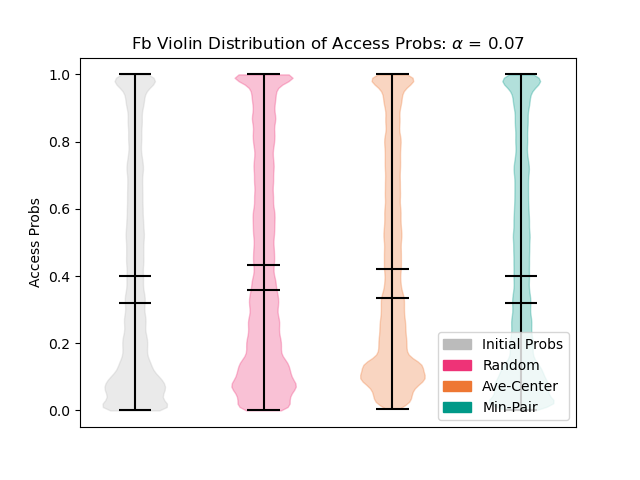}
		\includegraphics[width=.18\columnwidth]{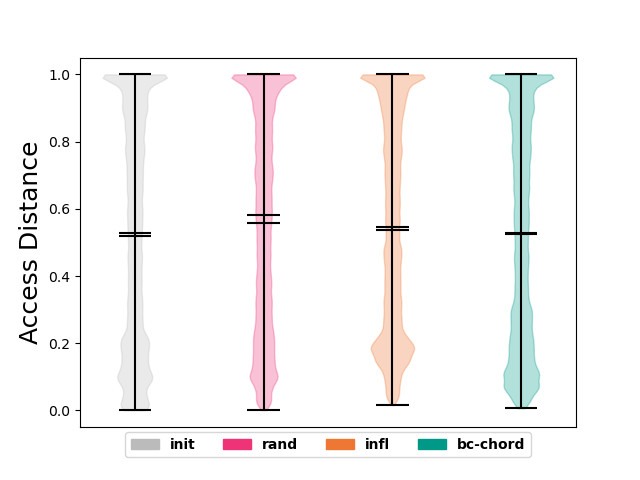}
		\includegraphics[width=.18\columnwidth]{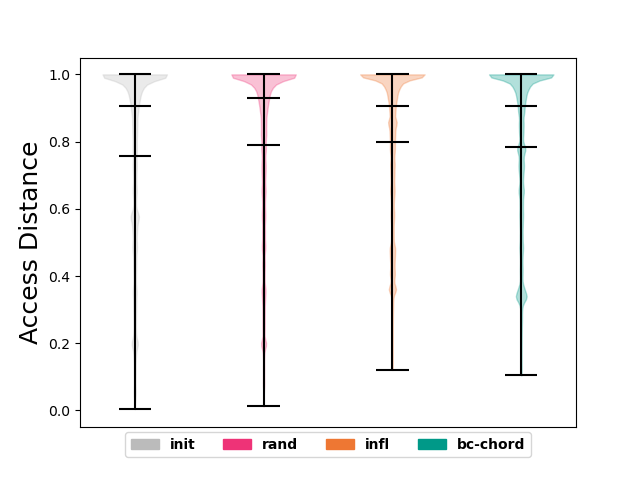}
		\includegraphics[width=.18\columnwidth]{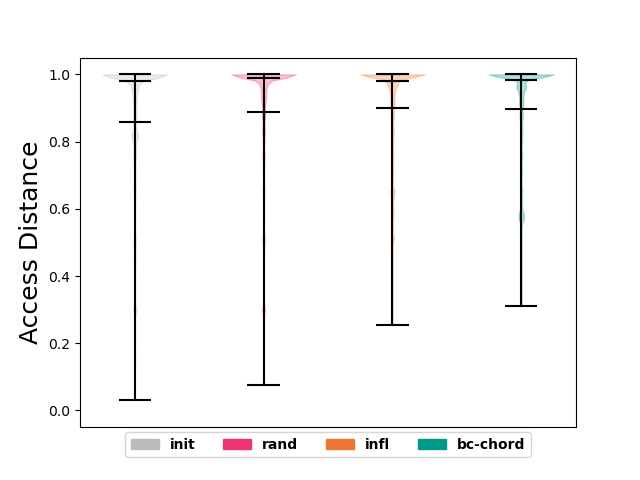}
		\includegraphics[width=.18\columnwidth]{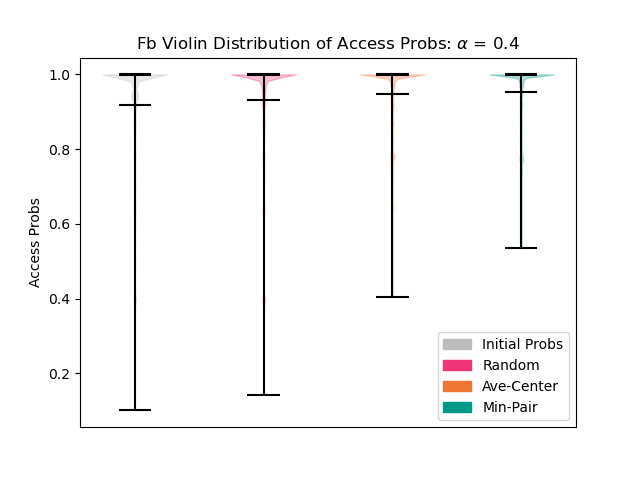}
		 \caption{Facebook}
	\end{subfigure}
	
	\begin{subfigure}[t]{\textwidth}
  		\includegraphics[width=.24\columnwidth]{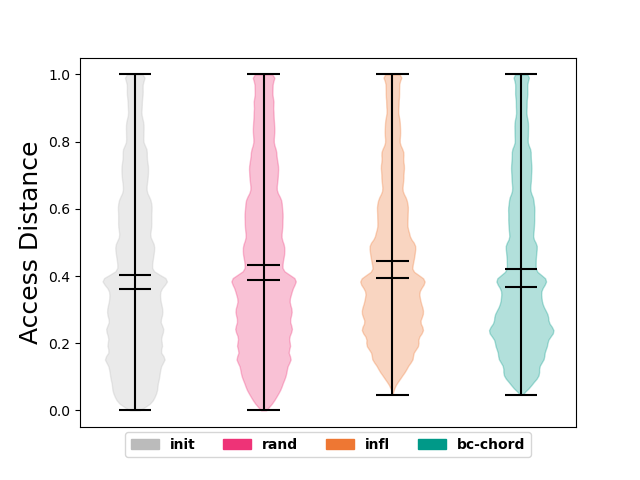}
		\includegraphics[width=.24\columnwidth]{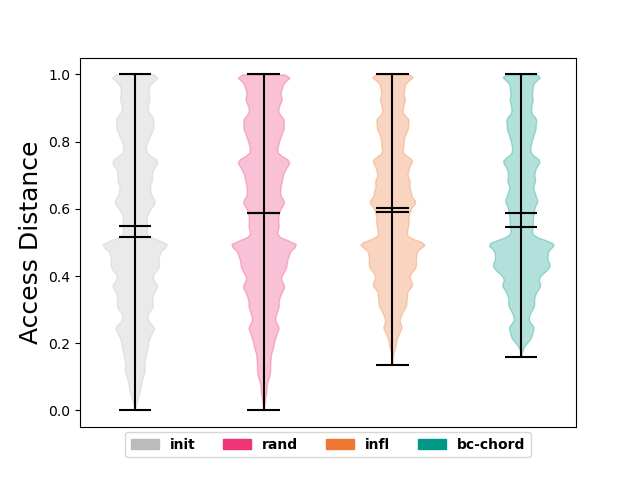}
		\includegraphics[width=.24\columnwidth]{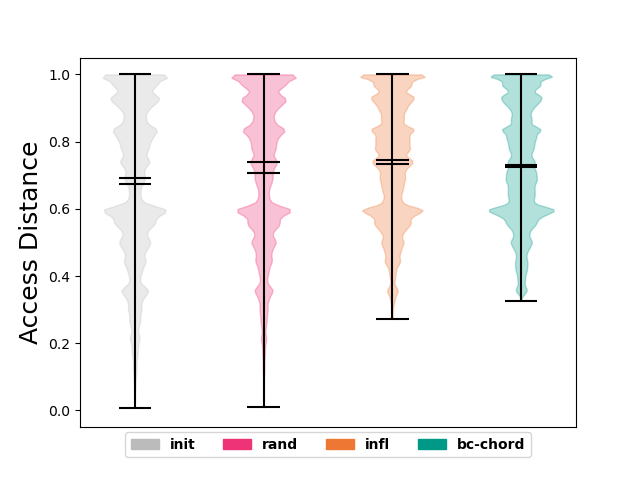}
		\includegraphics[width=.24\columnwidth]{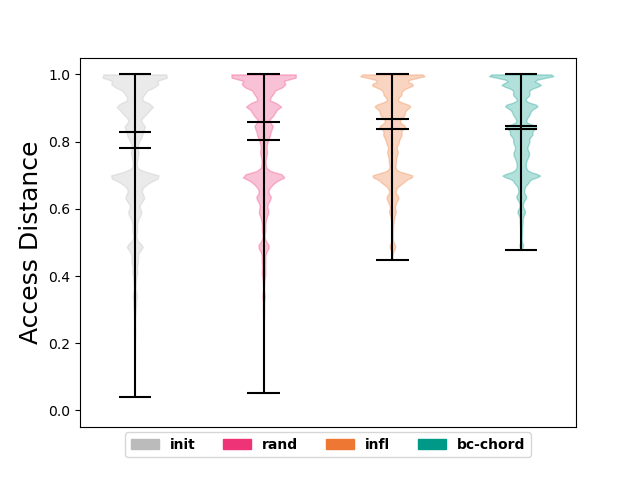}
		 \caption{Arxiv-3}
	\end{subfigure}
	
	\begin{subfigure}[t]{\textwidth}
  		\includegraphics[width=.24\columnwidth]{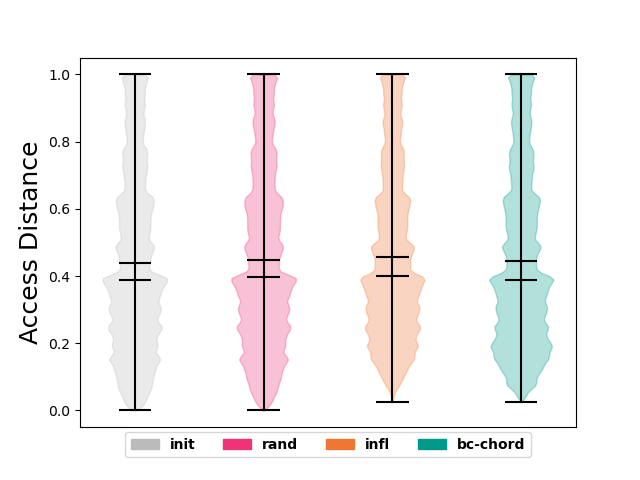}
		\includegraphics[width=.24\columnwidth]{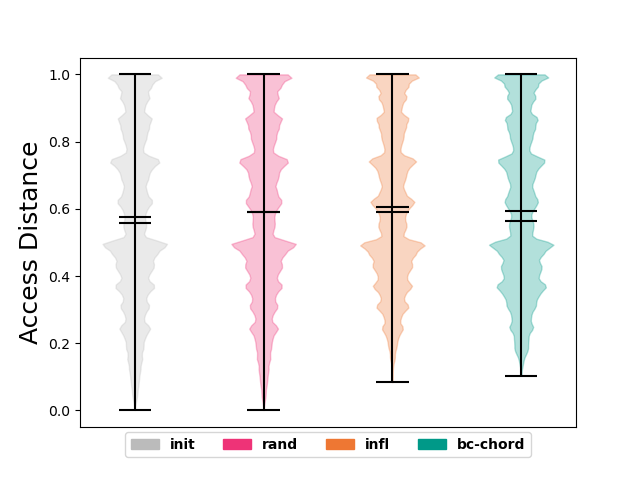}
		\includegraphics[width=.24\columnwidth]{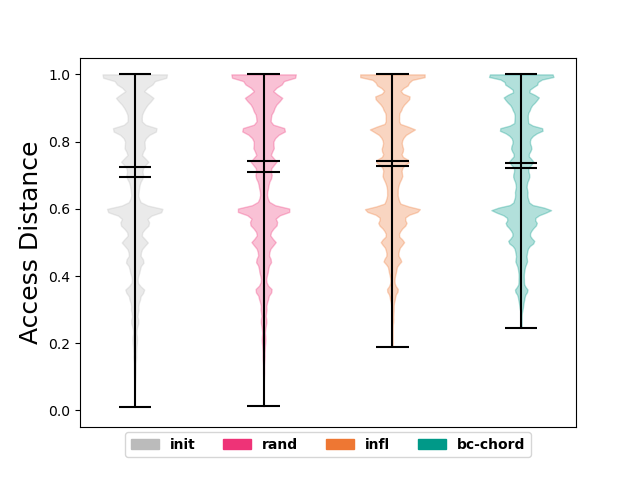}
		\includegraphics[width=.24\columnwidth]{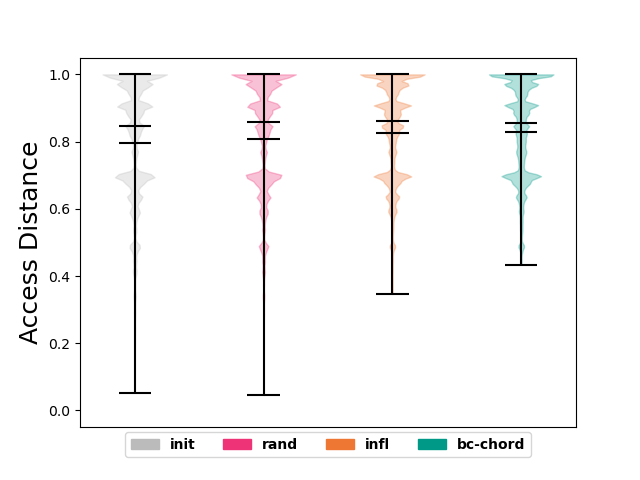}
		 \caption{Arxiv-5}
	\end{subfigure}
	
	\caption{Shift in the distribution (Violin Plot) of all access distances.}
	\label{fig:shift-mindist}
\end{figure*}

\begin{figure*}
	\centering
	\begin{subfigure}[t]{\textwidth}
		\includegraphics[width=.18\columnwidth]{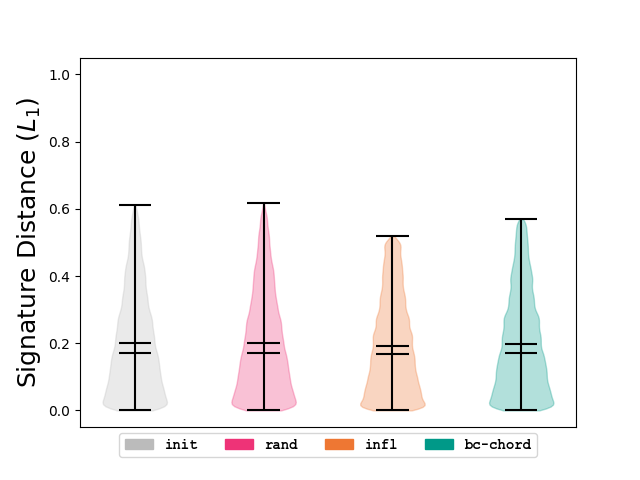}
		\includegraphics[width=.18\columnwidth]{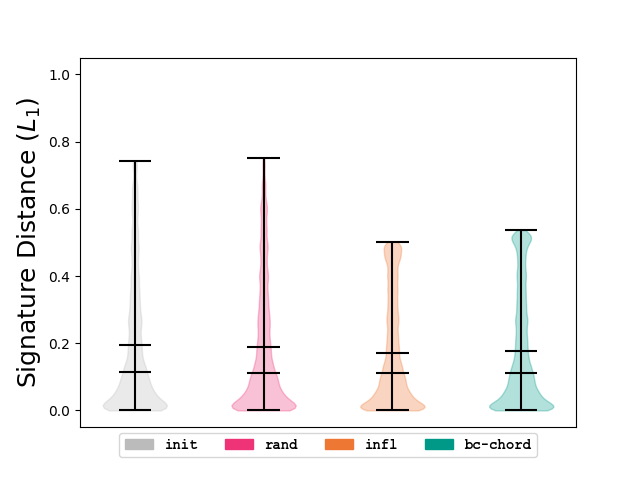}
		\includegraphics[width=.18\columnwidth]{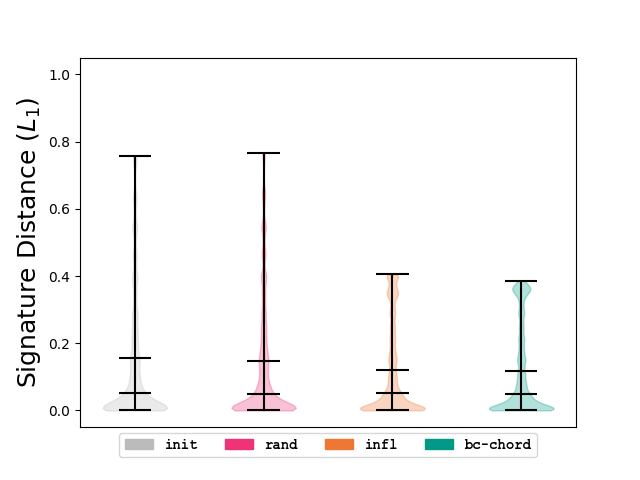}
		\includegraphics[width=.18\columnwidth]{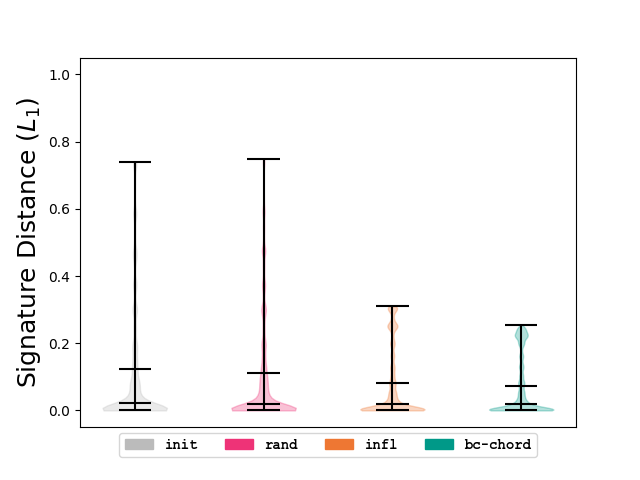}
		\includegraphics[width=.18\columnwidth]{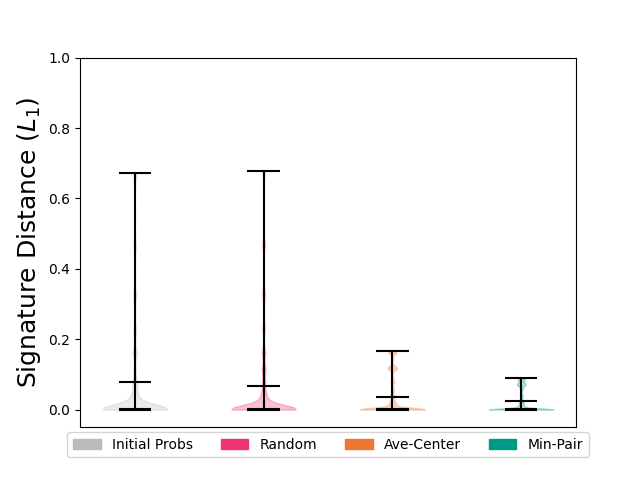}
		\caption{Email-EU}
	\end{subfigure}

	\begin{subfigure}[t]{\textwidth}
 		\includegraphics[width=.18\columnwidth]{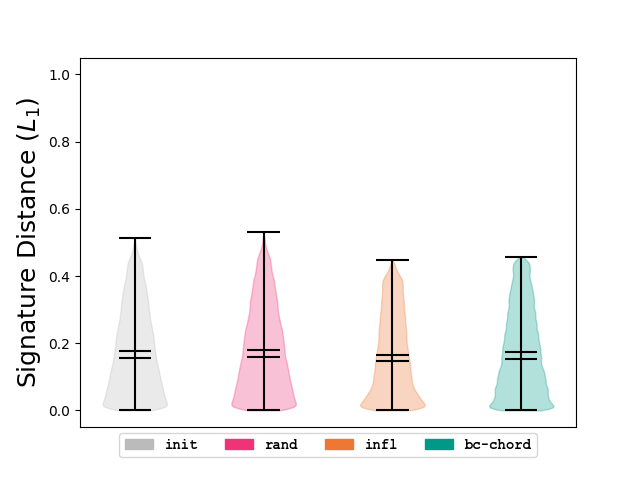}
		\includegraphics[width=.18\columnwidth]{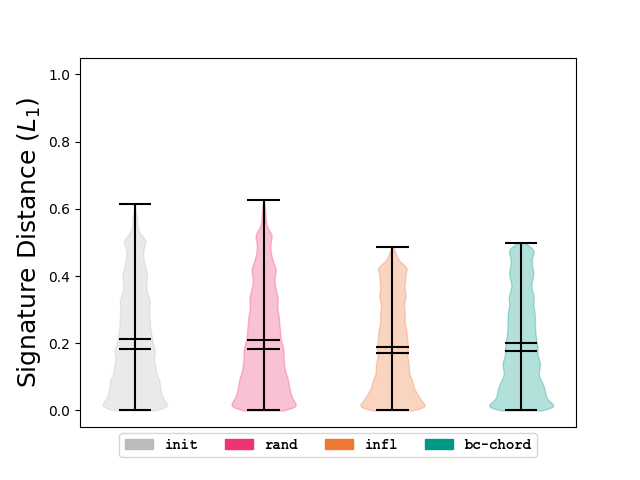}
 		\includegraphics[width=.18\columnwidth]{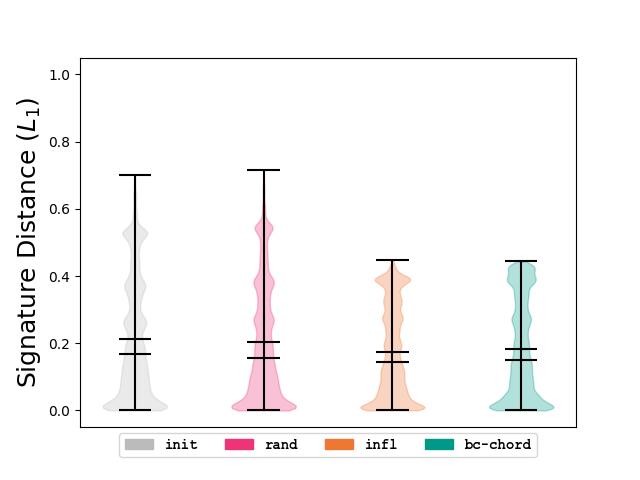}
		\includegraphics[width=.18\columnwidth]{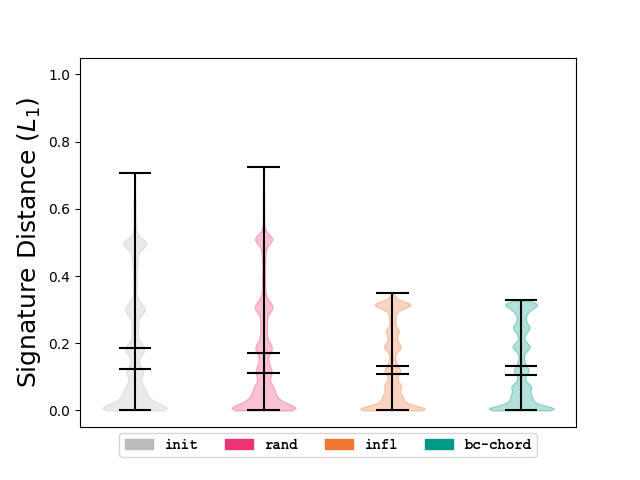}
		\includegraphics[width=.18\columnwidth]{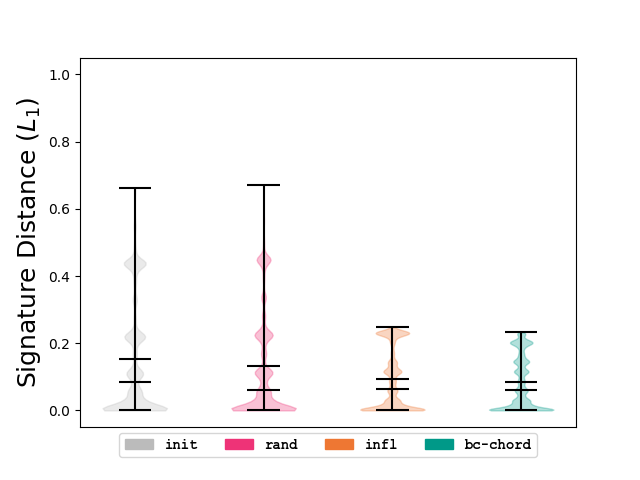}
		\caption{Email-arenas}
	\end{subfigure}

	\begin{subfigure}[t]{\textwidth}
  		\includegraphics[width=.18\columnwidth]{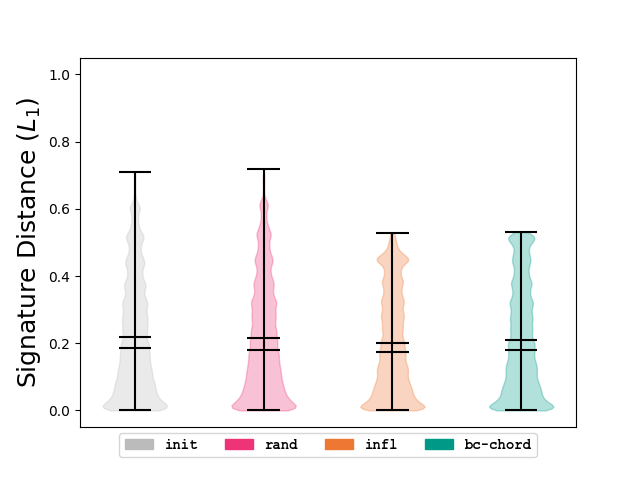}
		\includegraphics[width=.18\columnwidth]{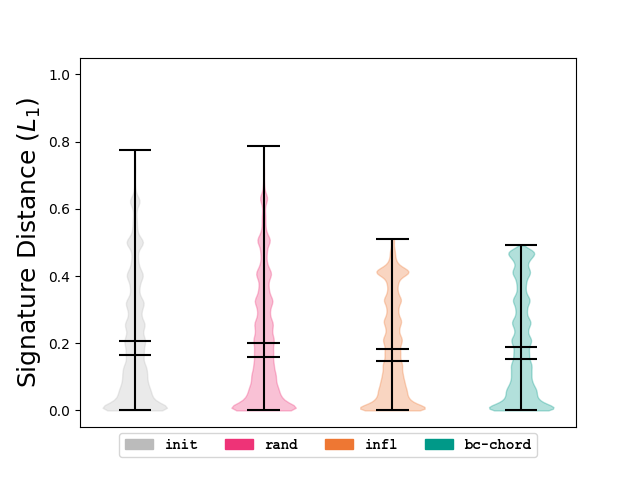}
		\includegraphics[width=.18\columnwidth]{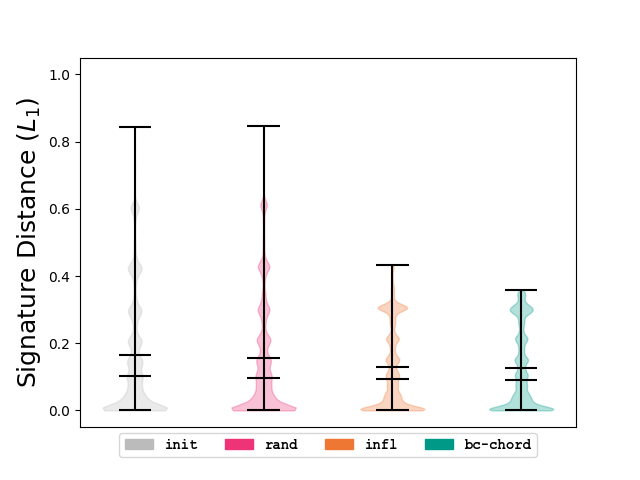}
		\includegraphics[width=.18\columnwidth]{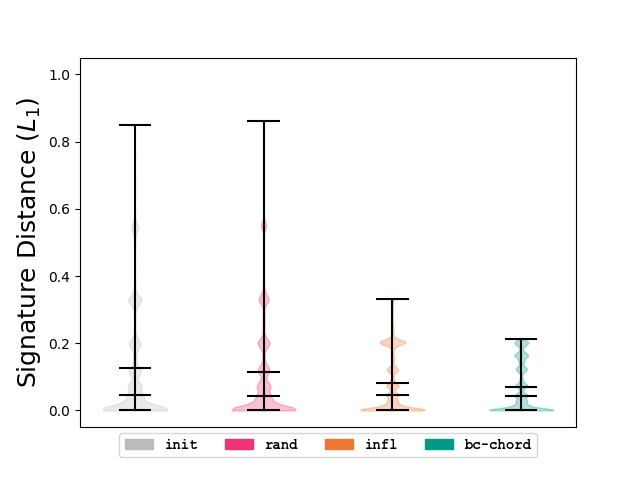}
		\includegraphics[width=.18\columnwidth]{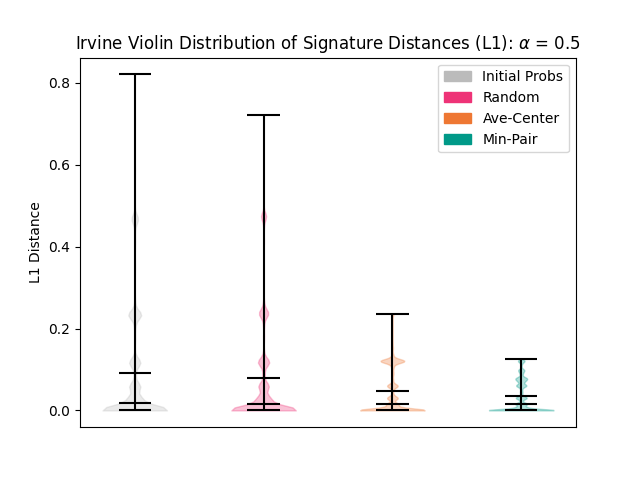}
		 \caption{Irvine}
	\end{subfigure}
	
	\begin{subfigure}[t]{\textwidth}
  		\includegraphics[width=.18\columnwidth]{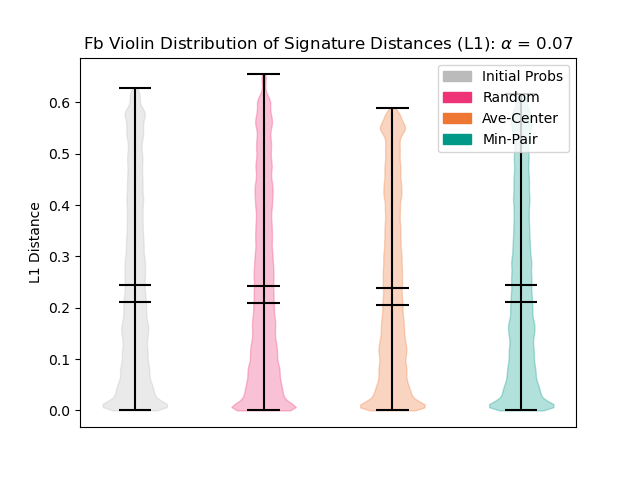}
		\includegraphics[width=.18\columnwidth]{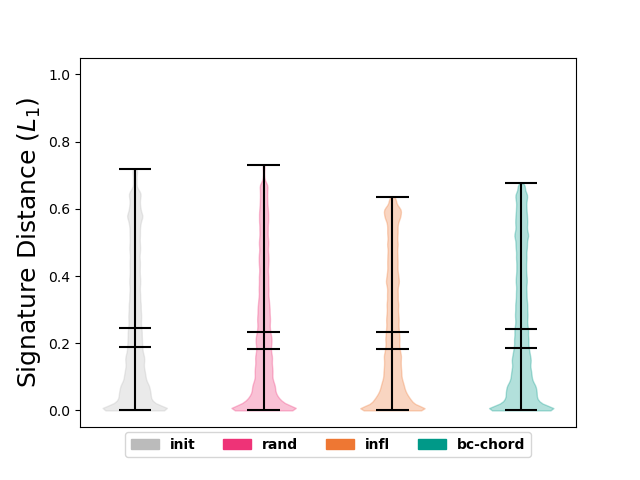}
		\includegraphics[width=.18\columnwidth]{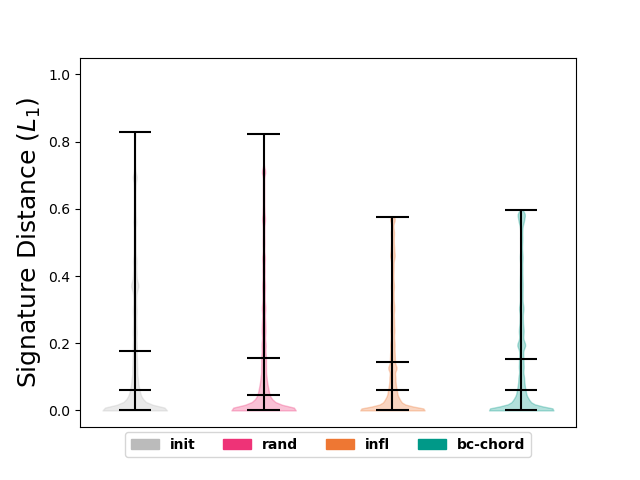}
		\includegraphics[width=.18\columnwidth]{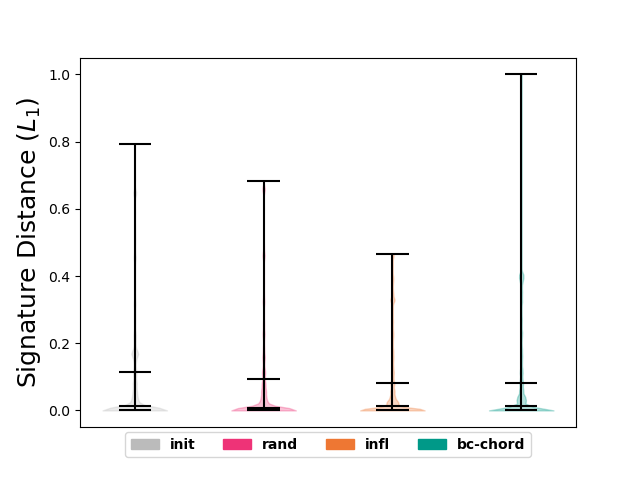}
		\includegraphics[width=.18\columnwidth]{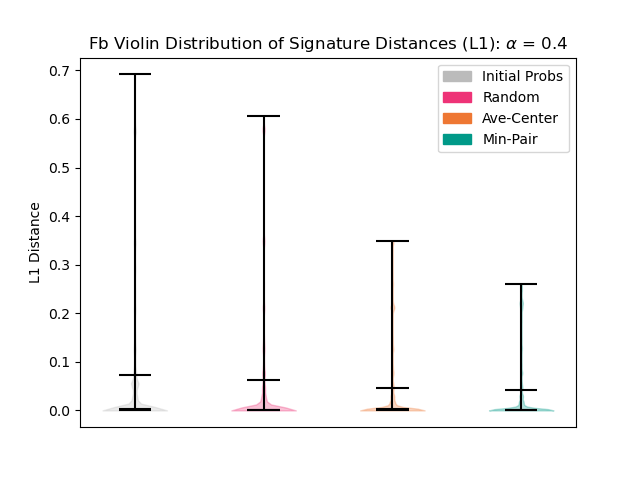}
		 \caption{Facebook}
	\end{subfigure}
	
	\begin{subfigure}[t]{\textwidth}
  		\includegraphics[width=.24\columnwidth]{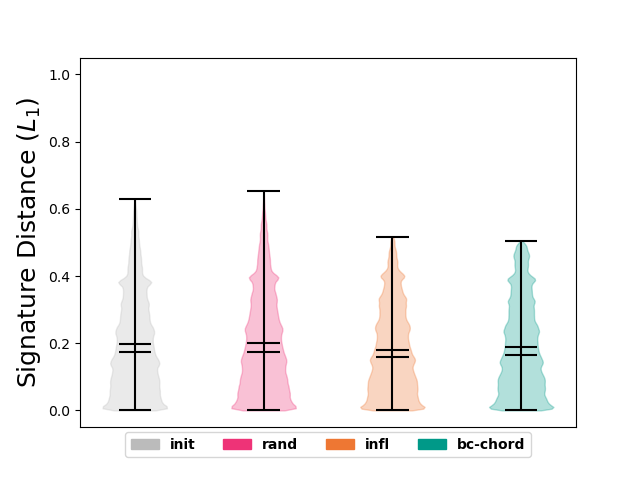}
		\includegraphics[width=.24\columnwidth]{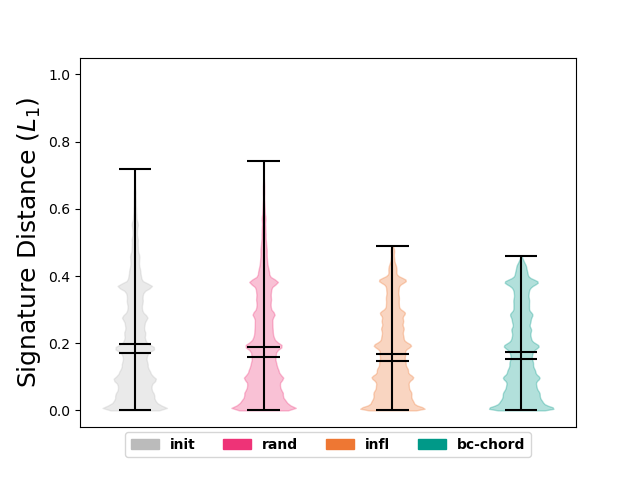}
		\includegraphics[width=.24\columnwidth]{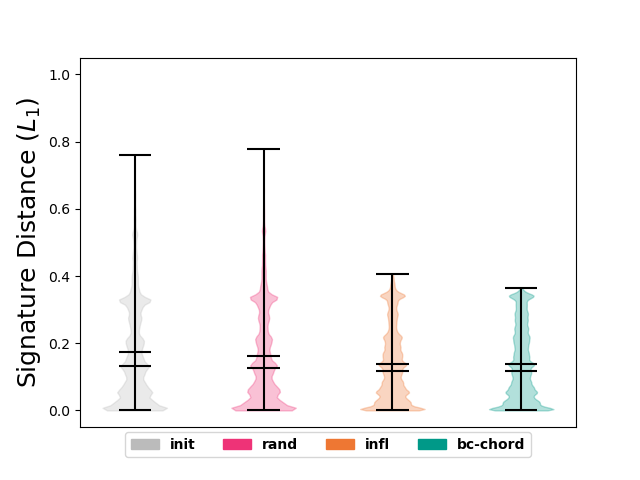}
		\includegraphics[width=.24\columnwidth]{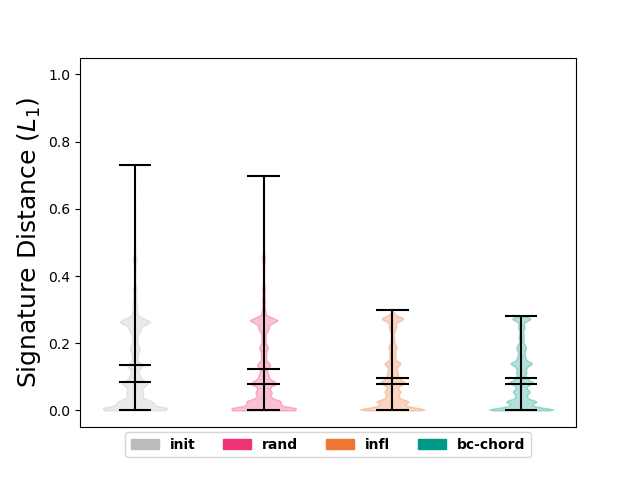}
		 \caption{Arxiv-3}
	\end{subfigure}
	
	\begin{subfigure}[t]{\textwidth}
  		\includegraphics[width=.24\columnwidth]{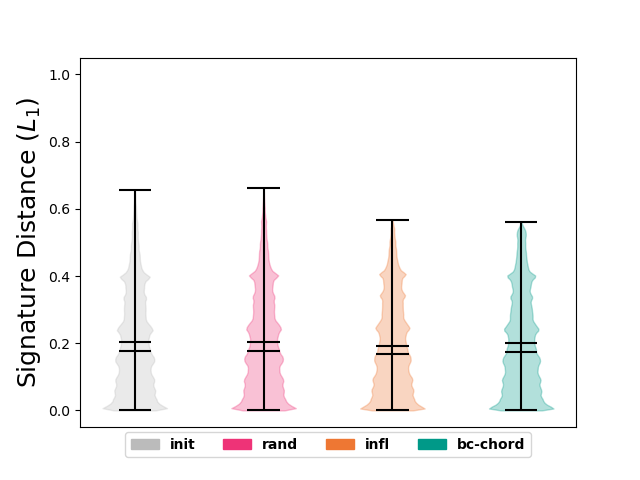}
		\includegraphics[width=.24\columnwidth]{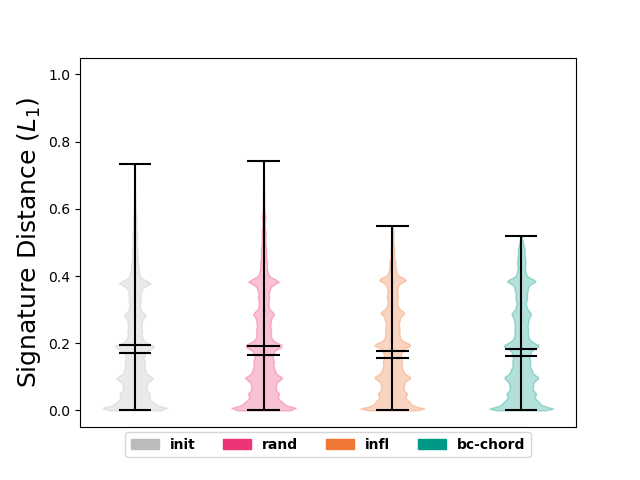}
		\includegraphics[width=.24\columnwidth]{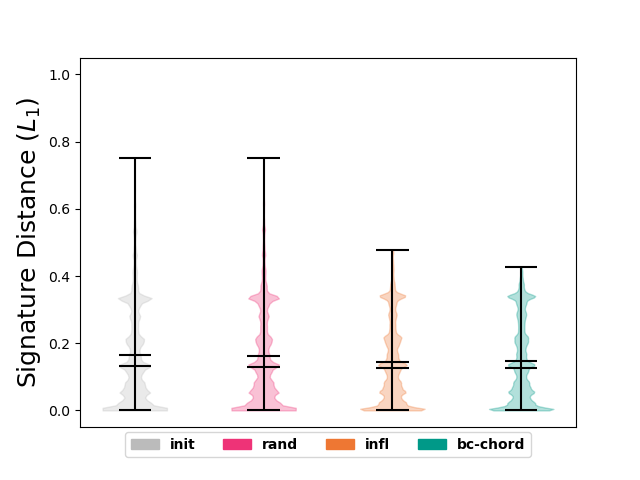}
		\includegraphics[width=.24\columnwidth]{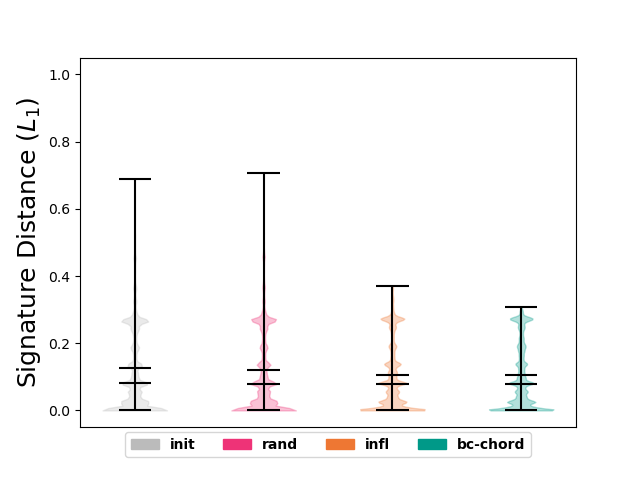}
		 \caption{Arxiv-5}
	\end{subfigure}

	\caption{Shift in the distribution (Violin plot) of signature manhattan distances.}
	\label{fig:sig-dist-manhat}
\end{figure*}
